# Supplementary material for: Learn Locally, Correct Globally: A Distributed Algorithm for Training Graph Neural Networks
Source: arXiv:2111.08202 source file (2022-03-13)
Supplement: Supplementary file 1 [file 01.notation.tex]

\section{Summary of notation}

We summarized all notations used throughout the paper in Table~\ref{table:notations}.

\begin{table*}[h]
\caption{Summary of notations used in this paper}
\label{table:notations}
\centering
\begin{tabularx}{\textwidth}{@{}sX@{}} \toprule
    $\mathcal{G}=(\mathcal{V},\mathcal{E})$  & $\mathcal{G}$ denotes the graph consist of set of $N=|\mathcal{V}|$ nodes and $M=|\mathcal{E}|$ edges. \\ \hline
    $\mathbf{A}, \mathbf{A}_p$ & $\mathbf{A}$ denotes the adjacency matrix corresponding to the graph $\mathcal{G}$, similarly $\mathbf{A}_p$ is the adjacency of subgraph on worker $p$ \\ \hline
    $\mathbf{D}$ & Denotes the degree matrix corresponding to the graph $\mathcal{G}$. \\ \hline
    $\mathbf{L}$, $\mathbf{L}^{p}$ & $\mathbf{L}$ denotes the full Laplacian matrix calculated by $\mathbf{L}=\mathbf{D}^{-1/2}\mathbf{A}\mathbf{D}^{-1/2}$ and $\mathbf{L}^{p}$ is the Laplacian matrix for the local subgraph on worker $p$. \\ \hline
    $\mathbf{X}$, $\bm{x}_i$ & $\mathbf{X}$ denotes the node feature matrix for all $N$ nodes where $\mathbf{X}=[\bm{x}_1,\ldots,\bm{x}_N]$. \\ \hline
    $\mathbf{Y}, \bm{y}_i$ & $\mathbf{Y}$ denotes the stacked label features and $\bm{y}_i$ denotes the label vector in $\mathbb{R}^C$. For example, in binary classification task, $\bm{y}_i\in\mathbb{R}^C$ is a one-hot vector with $C=2$.   \\ \hline
    $\mathbf{H}^{(\ell)},\mathbf{Z}^{(\ell)}$ & $\mathbf{Z}^{(\ell)}$ denotes the node feature matrix for the $\ell$th layer before activation and $\mathbf{H}^{(\ell)} = \sigma(\mathbf{Z}^{(\ell)})$ denotes the node feature matrix after the $\ell$th layer. \\ \hline
    $\mathbf{W}^{(\ell)}, \bm{\theta}$ $\mathbf{W}_p^{(\ell)}, \bm{\theta}_p$ & {$\mathbf{W}^{(\ell)}$ denotes the weight matrix for the $\ell$th graph convolution layer, $\bm{\theta}:=\{\mathbf{W}^{(1)},\ldots,\mathbf{W}^{(L)}\}$ denotes the stacked parameters. Per worker weight matrix and parameters are defined respectively.} \\ \hline
    $\kappa$ & The residual error as a result of applying naive parameter averaging in distributed GCNs. \\ \hline
    $P, T, K, S $ & $P$ denotes the number of local workers and $T$ is the total number of SGD updates. $K$ denotes the number of local worker iterations and $S$ is number of server correction iterations per epoch.\\ \hline
    $\mathcal{L}(\bm{\theta}), \mathcal{L}_p^\text{local}(\bm{\theta})$ $\mathcal{L}_p^\text{full}(\bm{\theta})$ &  $\mathcal{L}(\bm{\theta})$ denotes the objective on the global graph, $\mathcal{L}_p^\text{local}(\bm{\theta})$ denotes the local objective on the local subgraph and $\mathcal{L}_p^\text{full}(\bm{\theta})$ is the local objective with access to the global graph. \\ \hline
    $\mathcal{N}{(v_i)}, \mathcal{N}_p{(v_i)}$ & Denote the neighbor of node $v_i$ on the global graph and local graph respectively \\ \hline
    $\eta, \gamma$ & Learning rate on the server and local workers, respectively.  \\ \hline 
    $\sigma(\cdot)$ & $\sigma(\cdot)$ is the activation function, e.g., ReLU function. \\\hline
    $\phi(\cdot, \bm{y}_i)$ & $\phi(\cdot,\bm{y}_i)$ is the loss function, e.g., cross-entropy loss
    \begin{equation*}
    \phi(\bm{z}_i, \bm{y}_i) = -\log\left(\frac{\exp( \bm{z}_i^\top {\bm{y}_i})}{\sum_{j=1}^C \exp([\bm{z}_i]_j))}\right),
    \end{equation*}
    where label vector $\bm{y}_i$ is a one-hot vector. \\
    \bottomrule
\end{tabularx}
\end{table*}
