# Supplementary material for: Learn Locally, Correct Globally: A Distributed Algorithm for Training Graph Neural Networks
Source: arXiv:2111.08202 source file (2022-03-13)
Supplement: Supplementary file 2 [file 04.gradient_difference.tex]

\clearpage
\section{Proof of Lemma~\ref{lemma:local_machine_structure_err}}

Let consider a single layer GNN with the loss $\mathcal{L}(\bm{\theta})$ and the gradient $\nabla \mathcal{L}(\bm{\theta})$ computed by 
\begin{equation}
    \begin{aligned}
    \mathcal{L}(\bm{\theta}) &= \frac{1}{N}\sum_{i\in\mathcal{V}} \ell(\mathbf{h}_i, y_i),~
    \mathbf{h}_i = \mathbf{W}^\top \sum_{j \in \mathcal{V}} L_{i,j} \mathbf{x}_j,~\\
    \nabla \mathcal{L}(\bm{\theta}) &= \frac{1}{N}\sum_{i\in\mathcal{V}} \frac{\partial\ell(\mathbf{h}_i, y_i)}{\partial \mathbf{h}_i} \Big( \sum_{j \in \mathcal{V}} L_{i,j} \mathbf{x}_j \Big).
    \end{aligned}
\end{equation}

When each local machine has access to the full graph structure and all other node features and suppose each local machine has the same number of nodes, we have 
\begin{equation}
    \nabla \mathcal{L}(\bm{\theta}) = \frac{1}{P}\sum_{p=1}^P \nabla \mathcal{L}_p^\text{full}(\bm{\theta}),~
    \nabla \mathcal{L}_p^\text{full} (\bm{\theta}) = \frac{P}{N}\sum_{i\in\mathcal{V}_p} \frac{\partial\ell(\mathbf{h}_i, y_i)}{\partial \mathbf{h}_i} \Big( \sum_{j \in \mathcal{V}} L_{i,j} \mathbf{x}_j \Big).
\end{equation}

However, in practice each local machine only have access to the node feature and graph structure on its local machine, i.e.,
\begin{equation}
    \nabla \mathcal{L}_p^\text{local} (\bm{\theta}) = \frac{P}{N}\sum_{i\in\mathcal{V}_p} \frac{\partial\ell(\tilde{\mathbf{h}}_i, y_i)}{\partial \tilde{\mathbf{h}}_i} \Big( \sum_{j \in \mathcal{V}_p} L_{i,j}^p \mathbf{x}_j \Big).
\end{equation}

Define the local neighbor of node $v_i$ on machine $p$ by 
\begin{equation}
    \mathcal{N}^p(v_i) = \{ v_j|(v_i, v_j) \in \mathcal{E}_p\}.
\end{equation}

Let consider the neighbor average aggregation, where $L_{i,j}^p = \frac{1}{|\mathcal{N}^p(v_i)|}$ and $L_{i,j} = \frac{1}{|\mathcal{N}(v_i)|}$, we can upper bound $\mathbb{E}[ \| \tilde{\mathbf{h}}_i - \mathbf{h}_i \| ]$ by
\begin{equation}\label{eq:one_layer_example_eq_1}
    \mathbb{E}[ \| \tilde{\mathbf{h}}_i - \mathbf{h}_i \| ] \leq \mathbb{E} \Big[ \Big\| \mathbf{W}^\top \sum_{j \in \mathcal{V}_p} L_{i,j}^\text{local} \mathbf{x}_j - \mathbf{W}^\top \sum_{j \in \mathcal{V}} L_{i,j} \mathbf{x}_j \Big\| \Big] \leq D_\sigma B_w.
\end{equation}

To upper bound $\mathbb{E}[\| \nabla \mathcal{L}_p^\text{local}(\bm{\theta}) - \nabla \mathcal{L}_p^\text{full}(\bm{\theta}) \|^2]$, we have
\begingroup
\allowdisplaybreaks
    \begin{align*}
    & \mathbb{E}[\| \nabla \mathcal{L}_p^\text{local}(\bm{\theta}) - \nabla \mathcal{L}_p^\text{full}(\bm{\theta}) \|^2] \\
    &= \mathbb{E}\Big[\Big\| \frac{P}{N}\sum_{i\in\mathcal{V}_p} \frac{\partial\ell(\tilde{\mathbf{h}}_i, y_i)}{\partial \tilde{\mathbf{h}}_i} \Big( \sum_{j \in \mathcal{V}_p} L_{i,j}^p \mathbf{x}_j \Big) - \frac{P}{N}\sum_{i\in\mathcal{V}_p} \frac{\partial\ell(\mathbf{h}_i, y_i)}{\partial \mathbf{h}_i} \Big( \sum_{j \in \mathcal{V}} L_{i,j} \mathbf{x}_j \Big) \Big\|^2 \Big] \\
    %======
    &\leq 2 \mathbb{E} \Big[ \Big\| \frac{P}{N} \sum_{i\in\mathcal{V}_p} \frac{\partial\ell(\tilde{\mathbf{h}}_i, y_i)}{\partial \tilde{\mathbf{h}}_i} \Big( \sum_{j \in \mathcal{V}_p} L_{i,j}^p \mathbf{x}_j \Big) - \frac{P}{N}\sum_{i\in\mathcal{V}_p} \frac{\partial\ell(\mathbf{h}_i, y_i)}{\partial \mathbf{h}_i} \Big( \sum_{j \in \mathcal{V}_p} L_{i,j}^p \mathbf{x}_j \Big) \Big\|^2 \Big] \\
    &\quad + 2\mathbb{E} \Big[ \Big\| \frac{P}{N}\sum_{i\in\mathcal{V}_p} \frac{\partial\ell(\mathbf{h}_i, y_i)}{\partial \mathbf{h}_i} \Big( \sum_{j \in \mathcal{V}_p} L_{i,j}^p \mathbf{x}_j \Big) - \frac{P}{N}\sum_{i\in\mathcal{V}_p} \frac{\partial\ell(\mathbf{h}_i, y_i)}{\partial \mathbf{h}_i} \Big( \sum_{j \in \mathcal{V}} L_{i,j} \mathbf{x}_j \Big) \Big\|^2 \Big] \\
    %=======
    &\leq 2\mathbb{E} \Big[ \Big\| \frac{P}{N} \sum_{i\in\mathcal{V}_p} \Big( \frac{\partial\ell(\tilde{\mathbf{h}}_i, y_i)}{\partial \tilde{\mathbf{h}}_i} - \frac{\partial\ell(\mathbf{h}_i, y_i)}{\partial \mathbf{h}_i} \Big) \Big( \sum_{j \in \mathcal{V}_p} L_{i,j}^p \mathbf{x}_j \Big) \Big\|^2 \Big] \\
    &\quad + 2\mathbb{E} \Big[ \Big\| \frac{P}{N}\sum_{i\in\mathcal{V}_p} \frac{\partial\ell(\mathbf{h}_i, y_i)}{\partial \mathbf{h}_i} \Big( \sum_{j \in \mathcal{V}_p} L_{i,j}^p \mathbf{x}_j - \sum_{j \in \mathcal{V}} L_{i,j} \mathbf{x}_j \Big) \Big\|^2 \Big] \\
    %=======
    &\leq \frac{2P}{N} \sum_{i \in \mathcal{V}_p} \mathbb{E} \Big[ \Big\| \Big( \frac{\partial\ell(\tilde{\mathbf{h}}_i, y_i)}{\partial \tilde{\mathbf{h}}_i} - \frac{\partial\ell(\mathbf{h}_i, y_i)}{\partial \mathbf{h}_i} \Big) \Big( \sum_{j \in \mathcal{V}_p} L_{i,j}^p \mathbf{x}_j \Big) \Big\|^2 \Big] \\
    &\quad + \frac{2P}{N} \sum_{i \in \mathcal{V}_p} \mathbb{E} \Big[ \Big\| \frac{\partial\ell(\mathbf{h}_i, y_i)}{\partial \mathbf{h}_i} \Big( \sum_{j \in \mathcal{V}_p} L_{i,j}^p \mathbf{x}_j - \sum_{j \in \mathcal{V}} L_{i,j} \mathbf{x}_j \Big) \Big\|^2 \Big] \\
    %=======
    &\underset{(a)}{\leq} \frac{2P}{N} \sum_{i \in \mathcal{V}_p} L_\ell^2 \mathbb{E}[ \| \tilde{\mathbf{h}}_i - \mathbf{h}_i \|^2] \mathbb{E} \Big[ \Big\| \sum_{j \in \mathcal{V}_p} L_{i,j}^p \mathbf{x}_j \Big\|^2 \Big] \\
    &\quad + \frac{2P}{N} \sum_{i \in \mathcal{V}_p} \rho_\ell^2 \mathbb{E} \Big[ \Big\| \sum_{j \in \mathcal{V}_p} L_{i,j}^p \mathbf{x}_j - \sum_{j \in \mathcal{V}} L_{i,j} \mathbf{x}_j \Big\|^2 \Big],
\end{align*}
where $(a)$ is due to Lipschitz and smoothness assumption of loss function.

Recall $L_{i,j}^\text{local} = \frac{1}{|\mathcal{N}^\text{local}(v_i)|}$ and $L_{i,j} = \frac{1}{|\mathcal{N}(v_i)|}$, by plugging in Eq.~\ref{eq:one_layer_example_eq_1}, we can upper bound $\mathbb{E}[\| \nabla \mathcal{L}_p^\text{local}(\bm{\theta}) - \nabla \mathcal{L}_p^\text{full}(\bm{\theta}) \|^2]$ by
\begin{equation}
    \mathbb{E}[\| \nabla \mathcal{L}_p^\text{local}(\bm{\theta}) - \nabla \mathcal{L}_p^\text{full}(\bm{\theta}) \|^2] \leq 2 L_\ell^2 B_w^2 B_x^2 D_\sigma^2 + 2 \rho_\ell^2 D_\sigma^2.
\end{equation}
